# Supplementary material for: ProteinRPN: Towards Accurate Protein Function Prediction with Graph-Based Region Proposals
Source: arXiv:2409.00610 source file (2024-09-01)
Supplement: Supplementary file 1 [file Appendix.tex]

As before, each node's $k$-hop subgraph is treated as an anchor, with the node itself serving as the representative of the anchor. This reformulates the original graph $G$ into $G'(H', A)$, where each node in $G'$ represents a subgraph in $G$. Two parallel Graph Neural Network (GNN) layers process $G'$: the first predicts the likelihood of each anchor containing a functional site, while the second generates a vector that determines which nodes within the anchor's subgraph should be retained or pruned.

Anchors are assigned positive labels based on their Jaccard Similarity overlap with ground-truth annotations. Specifically, an anchor is considered positive if its Jaccard Similarity is higher than a predefined threshold of 0.7 and negative if it falls below 0.3. This dual-threshold method ensures clear differentiation between functionally relevant and irrelevant regions.

The optimization of the ProteinRPN is governed by a loss function that integrates both classification and regression tasks:
\[
\mathcal{L}(\{p_i\}, \{t_i\}) = \frac{1}{N_{\text{cls}}} \sum_{i} \mathcal{L}_{\text{cls}}(p_i, p_i^*) + \lambda \frac{1}{N_{\text{reg}}} \sum_{i} p_i^* \mathcal{L}_{\text{pruning}}(G_i, G_i^*)
\]
where:
\begin{itemize}
    \item $\mathcal{L}_{\text{cls}}(p_i, p_i^*)$ is the classification loss, computed as the binary cross-entropy between the predicted probability $p_i$ and the ground truth $p_i^*$, indicating the presence or absence of a functional site.
    \item $\mathcal{L}_{\text{pruning}}(G_i, G_i^*)$ assesses the pruning accuracy, calculated as the mismatch in the overlap between the pruned and the ground truth subgraphs.
    \item $\lambda$ is a balancing parameter that regulates the relative importance of the classification and pruning losses in the overall loss function. Experimentation with values ranging from 0.1 to 1 indicates that setting $\lambda = 1$ provides a balanced emphasis, optimizing both the identification of functional sites and the accuracy of their spatial delineation.
\end{itemize}

This structured loss function facilitates the precise refinement of both the prediction of functional sites and their boundaries within the protein structure. 
High-confidence anchors and their associated subgraphs are aggregated. Overlapping subgraphs with significant overlap are unified to form comprehensive predictions of functional annotations. Firstly, anchors that have a high chance of containing a functional region are identified from the output of the functionality prediction unit (Probability of functionality>0.7). Within these anchors, the output of the pruning unit is inspected and the residues with high scores (Probability of retention>0.5) are retained as functional residues. Functional residues from nearby high confidence anchors are unified.

(where $D_E = 1280$ for ESM-1b)
